# Supplementary material for: On the nature of overcharging and charge inversion in electrical double layers
Source: arXiv:2212.00141 ancillary file (2023-10-05)
Supplement: Supplementary file 1 [file Supp_info_inversion.pdf]

## Supplemental Material for

### On the nature of overcharging and charge inversion in electrical double layers

Nikhil R. Agrawal,<sup>1</sup> Chao Duan,<sup>1</sup> and Rui Wang<sup>1,2,\*</sup>

<sup>1</sup>*Department of Chemical and Biomolecular Engineering,  
University of California, Berkeley, California 94720, USA*

<sup>2</sup>*Materials Sciences Division, Lawrence Berkeley National Laboratory, Berkeley, 94720, California, USA*

#### I. DERIVATION OF THE MODIFIED GAUSSIAN RENORMALIZED FLUCTUATION THEORY

We derive the theory for a system with a fixed charge distribution  $\rho_{\text{fix}}(\mathbf{r})$  in the presence of small mobile cations of valency  $q_+$  and anions of valency  $q_-$  dissolved in a solution of spatially varying dielectric permittivity  $\varepsilon(\mathbf{r})$ . The electrostatic Hamiltonian,  $\mathcal{H}$ , for this system can be written as

$$\mathcal{H} = \frac{e^2}{2} \int d\mathbf{r} d\mathbf{r}' \rho(\mathbf{r}) C(\mathbf{r}, \mathbf{r}') \rho(\mathbf{r}') \quad (1)$$

where  $\rho(\mathbf{r})$  is the total charge density at any position  $\mathbf{r}$

$$e\rho(\mathbf{r}) = e\rho_{\text{fix}}(\mathbf{r}) + e \int d\mathbf{r}' [q_+ h_+(\mathbf{r} - \mathbf{r}') \hat{c}_+(\mathbf{r}') - q_- h_-(\mathbf{r} - \mathbf{r}') \hat{c}_-(\mathbf{r}')] \quad (2)$$

$C$  is the Coulomb operator accounting for spatially varying dielectric

$$-\nabla \cdot [\epsilon(\mathbf{r}) \nabla C(\mathbf{r}, \mathbf{r}')] = \delta(\mathbf{r} - \mathbf{r}') \quad (3)$$

$\hat{c}_{\pm,s}(\mathbf{r}) = \sum_{i,s} \delta(\mathbf{r} - \mathbf{r}_i)$  are the particle density operator for the ions or solvent  $s$ ,  $e$  is elementary charge, and  $\epsilon(\mathbf{r}) = kT\varepsilon_0\varepsilon(\mathbf{r})/e^2$  is the scaled permittivity with  $\varepsilon_0$  the vacuum permittivity. Unlike mean-field Poisson-Boltzmann we consider the ion to be finite-sized, the function  $h_{\pm}(\mathbf{r} - \mathbf{r}')$  above is the charge distribution function for an ion centered at  $\mathbf{r}'$ .

Using the above defined electrostatic Hamiltonian  $\mathcal{H}$ , chemical potentials  $\mu_{\pm,s}$ , volumes  $v_{\pm,s}$ , and numbers  $n_{\pm,s}$  the grand canonical partition function,  $\Xi$ , could be written as

$$\Xi = \sum_{n_+, -, s=0}^{\infty} \frac{e^{\mu_+ n_+} e^{\mu_- n_-} e^{\mu_s n_s}}{n_+! n_-! n_s! v_+^{n_+} v_-^{n_-} v_s^{n_s}} \int \prod_{i=1}^{n_+} d\mathbf{r}_i \prod_{j=1}^{n_-} d\mathbf{r}_j \prod_{k=1}^{n_s} d\mathbf{r}_k \times \prod_{\mathbf{r}} \delta(1 - \hat{c}_+(\mathbf{r})v_+ - \hat{c}_-(\mathbf{r})v_- - \hat{c}_s(\mathbf{r})v_s) \exp(-\beta\mathcal{H}) \quad (4)$$

The dirac-delta functional above is added to include the excluded volume effect ensuring the total volume fraction of ions and solvent molecules is equal to 1. We next apply the usual Hubbard-Stratonovich transformation (HST) and Identity transformation (IT) on Eq. 4 to change the particle variables to field variables. HST introduces a field variable for electrostatic potential,  $\phi(\mathbf{r})$ , coupled with ion density  $\rho(\mathbf{r})$ . IT when applied on the functional delta introduces a field variable  $\xi(\mathbf{r})$  accounting for the incompressibility condition. The resulting expression for  $\Xi$  is

$$\Xi = \frac{1}{Z_0} \int D\phi \int D\xi (\exp[-L[\phi, \xi]]), \text{ where} \quad (5)$$

$$Z_0 = \int D\phi \exp \left[ -\frac{1}{2} \int d\mathbf{r} \epsilon (\nabla \phi)^2 \right] \text{ and } L = \int d\mathbf{r} \left[ \frac{1}{2} \epsilon (\nabla \phi)^2 + i\rho_{\text{fix}}\phi - \sum_{j=+, -} \lambda_j e^{-iq_j \int d\mathbf{r}' h_j(\mathbf{r}-\mathbf{r}') \phi(\mathbf{r}') - iv_j \xi} - \lambda_s e^{-iv_s \xi} - i\xi \right]$$

and  $\lambda_{j,s} = \frac{e^{\mu_{j,s}}}{v_{j,s}}$  is the fugacity which would later be determined using the given bulk concentration of ions and solvent molecules. The exact solution to  $\Xi$  is impossible and hence to get its best possible estimate we need to invoke

---

\* email: [ruiwang325@berkeley.edu](mailto:ruiwang325@berkeley.edu)

some approximations. The integral over  $\xi(\mathbf{r})$  is approximated using the saddle point method yielding the following expression

$$v_+ \lambda_+ e^{-iq_+ \hat{h}_+ \phi - v_+ \eta} + v_- \lambda_- e^{iq_- \hat{h}_- \phi - v_- \eta} + v_s \lambda_s e^{-v_s \eta} - 1 = 0 \quad (6)$$

where  $-i\eta(\mathbf{r})$  is the saddle point value of  $\xi(\mathbf{r})$ .  $\hat{h}_\pm \phi = \int d\mathbf{r}' h_\pm(\mathbf{r} - \mathbf{r}') \phi(\mathbf{r}')$ , is a short-hand notation denoting local spatial averaging of  $\phi$  by the charge distribution function. The partition function is now simplified to

$$\Xi = \frac{1}{Z_0} \int D\phi \exp \left\{ - \int d\mathbf{r} \left[ \frac{1}{2} \epsilon(\nabla \phi)^2 + i\rho_{\text{fix}} \phi - \lambda_+ e^{-iq_+ \hat{h}_+ \phi - v_+ \eta} - \lambda_- e^{iq_- \hat{h}_- \phi - v_- \eta} - \lambda_s e^{-v_s \eta} - \eta \right] \right\} \quad (7)$$

Taking the saddle-point approximation on  $\phi$  in the above equation will lead to the modified Poisson-Boltzmann theory with excluded volume effect but no ion correlations. To account for the correlations in a non-perturbative manner we estimate the integral in  $\phi$  using a variational procedure. The grand free energy  $\mathcal{W}$  is bounded from above using the Gibbs-Feynman-Bogoliubov (GFB) bound, where we took the reference action to be of the Gaussian form centered around the mean electrostatic potential,  $-i\psi$ . The corresponding equations read as

$$\mathcal{W}(-\mathcal{L}[\phi]) = -\ln \Xi \leq -\ln \Xi_{ref} + \langle \mathcal{L}[\phi] - \mathcal{L}_{ref}[\phi] \rangle_{ref} \quad (8)$$

$$\mathcal{L}_{ref} = \frac{1}{2} \int d\mathbf{r} d\mathbf{r}' [\phi(\mathbf{r}) + i\psi(\mathbf{r})] G(\mathbf{r}, \mathbf{r}') [\phi(\mathbf{r}') + i\psi(\mathbf{r}')] \quad (9)$$

The choice of a Gaussian reference action allows the derivation of an analytical expression for the r.h.s of Eq. 8. The detailed derivations are given in Ref. [1–3]. The resulting expression for the variational free energy is

$$\begin{aligned} \mathcal{W}_{var} = -\ln \Xi = & -\frac{1}{2} \ln \left[ \frac{\det G}{\det C} \right] - \frac{1}{2} \int d\mathbf{r} d\mathbf{r}' [\det G^{-1}(\mathbf{r}, \mathbf{r}') - \det C^{-1}(\mathbf{r}, \mathbf{r}')] G(\mathbf{r}, \mathbf{r}') - \frac{1}{2} \int d\mathbf{r} [\epsilon(\mathbf{r}) (\nabla \psi(\mathbf{r}))^2] \\ & - \int d\mathbf{r} [\lambda_+ e^{-q_+ \psi - u_+ - v_+ \eta} + \lambda_- e^{q_- \psi - u_- - v_- \eta} + \lambda_s e^{-v_s \eta} + \eta - \rho_{\text{fix}} \psi] \end{aligned} \quad (10)$$

$$u_\pm(\mathbf{r}) = \frac{q_\pm^2}{2} \int d\mathbf{r}' d\mathbf{r}'' h_\pm(\mathbf{r} - \mathbf{r}') G(\mathbf{r}', \mathbf{r}'') h_\pm(\mathbf{r}'' - \mathbf{r}) \quad (11)$$

where  $u_\pm$  is the self energy of ions, and  $G$  is the correlation function corresponding to the reference action. To get the best estimate of grand free energy we do a functional minimization of  $\mathcal{W}$  with respect to  $G$  and  $\psi$  giving us the following set of self-consistent equations

$$-\nabla_{\mathbf{r}'} \cdot [\epsilon(\mathbf{r}') \nabla_{\mathbf{r}'} G(\mathbf{r}', \mathbf{r}'')] + \int d\mathbf{r}_1 d\mathbf{r}_2 \sum_{j=+,-} q_j^2 h_j(\mathbf{r}' - \mathbf{r}_1) h_j(\mathbf{r}_1 - \mathbf{r}_2) c_j(\mathbf{r}_1) G(\mathbf{r}_2, \mathbf{r}'') = \delta(\mathbf{r}', \mathbf{r}'') \quad (12)$$

$$-\nabla \cdot [\epsilon(\mathbf{r}) \nabla \psi(\mathbf{r})] = \rho_{\text{fix}}(\mathbf{r}) + q_+ c_+(\mathbf{r}) - q_- c_-(\mathbf{r}) \quad (13)$$

$$c_\pm(\mathbf{r}) = \lambda_\pm \exp[-q_\pm \psi(\mathbf{r}) - u_\pm(\mathbf{r}) - v_\pm \eta(\mathbf{r})] \quad (14)$$

$$c_s(\mathbf{r}) = \lambda_s \exp[-v_s \eta(\mathbf{r})] \quad (15)$$

For simplicity, we approximate the  $h$  inside the integral as a dirac delta function for the purpose of calculating the correlation function, giving us the following equation for  $G$

$$-\nabla_{\mathbf{r}'} \cdot [\epsilon(\mathbf{r}') \nabla_{\mathbf{r}'} G(\mathbf{r}', \mathbf{r}'')] + 2I(\mathbf{r}') G(\mathbf{r}', \mathbf{r}'') = \delta(\mathbf{r}', \mathbf{r}'') \quad (16)$$

where  $2I(\mathbf{r}') = \epsilon(\mathbf{r}') \kappa^2(\mathbf{r}') = c_+(\mathbf{r}') q_+^2 + c_-(\mathbf{r}') q_-^2$  is the spatially varying ionic strength.

An expression for  $\eta(\mathbf{r})$  in terms of bulk concentrations of ions and chemical potential of solvent can be derived by combining Eq. 15 with saddle-point condition for field  $\xi(\mathbf{r})$  given in Eq. 6. The corresponding incompressibility condition looks like

$$v_+ c_+(\mathbf{r}) + v_- c_-(\mathbf{r}) + v_s c_s(\mathbf{r}) = 1 \quad (17)$$

Finally, for an electrically neutral solution, the boundary conditions for  $\psi$  are  $(d\psi/dz)_{z=0} = -\sigma/\epsilon_S$  and  $\psi(z=L) = 0$ .

## II. DECOMPOSITION OF THE CORRELATION FUNCTION

To solve for the spatially varying self-energy  $u_{\pm}(\mathbf{r})$  we need to resolve the correlation function  $G(\mathbf{r}, \mathbf{r}')$  at the length scale of both ion size and interfacial width. This dual-length scale problem is numerically intractable. In our previous work[4], we developed a formulation to handle this duality by writing the self-energy of any ion in the interface as

$$u_{\pm}(\mathbf{r}) = \frac{q_{\pm}^2}{2} \int d\mathbf{r}' d\mathbf{r}'' h_{\pm}(\mathbf{r} - \mathbf{r}') G_s(\mathbf{r}', \mathbf{r}'') h_{\pm}(\mathbf{r}'' - \mathbf{r}) + \frac{q_{\pm}^2}{2} G_1(\mathbf{r}, \mathbf{r}) \quad (18)$$

where the differential equation for  $G_s$ , the short-range contribution to the correlation function, is

$$-\epsilon(\mathbf{r}) \nabla_{\mathbf{r}'}^2 G_s(\mathbf{r}', \mathbf{r}'') + 2I(\mathbf{r}) G_s(\mathbf{r}', \mathbf{r}'') = \delta(\mathbf{r}', \mathbf{r}'') \quad (19)$$

The differential equation for  $G_1$ , the long-range contribution to the correlation function, is

$$-\nabla_{\mathbf{r}'} \cdot [\epsilon(\mathbf{r}') \nabla_{\mathbf{r}'} G_1(\mathbf{r}', \mathbf{r}'')] + 2I(\mathbf{r}') G_1(\mathbf{r}', \mathbf{r}'') = S(\mathbf{r}', \mathbf{r}'') \quad (20)$$

and the non-local source term  $S$  is

$$S(\mathbf{r}', \mathbf{r}'') = \nabla_{\mathbf{r}'} \cdot (\epsilon(\mathbf{r}') - \epsilon(\mathbf{r})) \nabla_{\mathbf{r}'} G_s(\mathbf{r}', \mathbf{r}'') - 2(I(\mathbf{r}') - I(\mathbf{r})) G_s(\mathbf{r}', \mathbf{r}'')$$

The first term in Eq. 18,  $u_{\pm,s}(\mathbf{r})$  has an analytical solution given by

$$u_{\pm,s}(\mathbf{r}) = \frac{q_{\pm}^2}{8\pi\epsilon(\mathbf{r})a_{\pm}} - \frac{q_{\pm}^2 \kappa(\mathbf{r})}{8\pi\epsilon(z)} \exp\left(\frac{a_{\pm}^2 \kappa(\mathbf{r})^2}{\pi}\right) \operatorname{erfc}\left(\frac{a_{\pm} \kappa(\mathbf{r})}{\sqrt{\pi}}\right) \quad (21)$$

To solve for the second term in Eq. 18 for a planar double layer next to a uniformly charged surface, we take advantage of symmetry in  $x - y$  directions parallel to the interface. We can write  $G_1$  and  $G_s$  in cylindrical coordinates  $(r, \theta, z)$  and then apply Fourier transform in  $r$  and  $\theta$  directions using the following definitions

$$G_{1,s}(r, z', z'') = \int_0^{\infty} \frac{J_0(sr)}{2\pi} \hat{G}_{1,s}(s, z', z'') s ds \quad (22)$$

where  $J_0$  is the zeroth order Bessel function. The corresponding Fourier transformed version of Equation 20 is

$$-\frac{\partial}{\partial z'} [\epsilon(z') \frac{\partial \hat{G}_l(s, z', z'')}{\partial z'}] + \epsilon(z') (\kappa^2(z') + s^2) \hat{G}_l(s, z', z'') = \hat{S}(s, z', z'') \quad (23)$$

where  $\hat{S}$  is

$$\hat{S}(s, z', z'') = \frac{\partial}{\partial z'} [(\epsilon(z') - \epsilon(z'')) \frac{\partial \hat{G}_s(s, z', z'')}{\partial z'}] - (\epsilon(z') (\kappa^2(z') + s^2) - \epsilon(z'') (\kappa^2(z'') + s^2)) \hat{G}_s(s, z', z'')$$

whereas the transformed version for Equation 19 is

$$-\frac{\partial}{\partial z'} [\frac{\partial \hat{G}_s(s, z', z'')}{\partial z'}] + (\kappa^2(z) + s^2) \hat{G}_s(s, z', z'') = \frac{\delta(z', z'')}{\epsilon(z)} \quad (24)$$

An analytical solution for  $\hat{G}_s$  exists and is given by

$$\hat{G}_s(s, z', z'') = \frac{e^{-p|z' - z''|}}{2p\epsilon(z)}, \text{ where } p = (s^2 + \kappa^2(z))^{1/2} \quad (25)$$

Although, one can directly solve Eqs. 23 and 25 using a finite difference scheme, in this work, we have used an easier and well-tested method [4, 5] to solve for  $G_1$ . In this alternative method, we rewrite the equation for  $u_{\pm}(\mathbf{r})$  using the functions  $G$  and  $G_s$  as shown below

$$u_{\pm}(\mathbf{r}) = u_{\pm,s}(\mathbf{r}) + \frac{q_{\pm}^2}{2} \lim_{\mathbf{r}', \mathbf{r}'' \rightarrow \mathbf{r}} (G(\mathbf{r}', \mathbf{r}'') - G_s(\mathbf{r}', \mathbf{r}'')) \quad (26)$$

We next define the free space correlation function  $G_o(\mathbf{r}', \mathbf{r}'')$  using local  $\epsilon(\mathbf{r})$  as

$$-\epsilon(\mathbf{r}) \nabla_{\mathbf{r}'}^2 G_o(\mathbf{r}', \mathbf{r}'') = \delta(\mathbf{r}', \mathbf{r}'') \quad (27)$$

Adding and subtracting  $G_o$  in Equation 26 yields

$$u_{\pm}(\mathbf{r}) = u_{\pm,s}(\mathbf{r}) + \frac{q_{\pm}^2}{2} \lim_{\mathbf{r}', \mathbf{r}'' \rightarrow \mathbf{r}} (G - G_o) + \frac{q_{\pm}^2}{2} \lim_{\mathbf{r}', \mathbf{r}'' \rightarrow \mathbf{r}} (G_o - G_s) \quad (28)$$

Solving for the limit in the third term leaves us with the following simplified expression for total self-energy  $u_{\pm}(\mathbf{r})$

$$u_{\pm}(\mathbf{r}) = u_{\pm,s}(\mathbf{r}) + \frac{q_{\pm}^2 \kappa(\mathbf{r})}{8\pi\epsilon(\mathbf{r})} + \frac{q_{\pm}^2}{2} \lim_{\mathbf{r}', \mathbf{r}'' \rightarrow \mathbf{r}} (G - G_o) \quad (29)$$

By applying a similar Fourier transform as Eq. 23 we can rewrite Eq. 16 and 27 as

$$-\frac{\partial}{\partial z'} [\epsilon(z') \frac{\partial \hat{G}(s, z', z'')}{\partial z'}] + \epsilon(z') (\kappa^2(z') + s^2) \hat{G}(s, z', z'') = \delta(z', z'') \quad (30)$$

$$-\frac{\partial^2 \hat{G}_o(s, z', z'')}{\partial z'^2} + s^2 \hat{G}_o(s, z', z'') = \frac{\delta(z', z'')}{\epsilon(z)} \quad (31)$$

Since  $J_o(sr)$  is equal to 1 for  $r = 0$ , the limit term of Eq. 29 becomes

$$\frac{q_{\pm}^2}{2} \lim_{\mathbf{r}', \mathbf{r}'' \rightarrow \mathbf{r}} (G - G_o) = \frac{q_{\pm}^2}{4\pi} \int_0^\infty (\hat{G}(s, z, z) - \hat{G}_o(s, z, z)) s ds \quad (32)$$

The boundary conditions (BCs) shown next are for the case of different but constant dielectric permittivity on either side of the charged plate. We denote the permittivity in the region  $z' < 0$  and  $z' > 0$  with  $\epsilon_s$  and  $\epsilon_p$ , respectively. For the solution domain  $z' \in [0, L]$ , the BCs for  $\hat{G}$  are

$$\epsilon_s \frac{\partial \hat{G}(s, z', z'')}{\partial z'} = s \epsilon_p \hat{G}(s, z', z'') \quad (33)$$

$$\frac{\partial \hat{G}(s, z', z'')}{\partial z'} = -(s^2 + \kappa_b^2)^{1/2} \hat{G}(s, z', z'') \quad (34)$$

which are applicable for  $z' = 0, z'' > 0$  and  $z' > L, z'' \leq L$  respectively. Here  $\kappa_b$  is the bulk screening constant. These BCs are derived using continuity of  $\hat{G}$  and its first derivative at the ends. Similarly the boundary conditions for  $\hat{G}_o$  are

$$\frac{\partial \hat{G}_o(s, z', z'')}{\partial z'} = s \hat{G}_o(s, z', z'') \quad (35)$$

$$\frac{\partial \hat{G}_o(s, z', z'')}{\partial z'} = -s \hat{G}_o(s, z', z'') \quad (36)$$

applied at  $z' = 0, z'' > 0$  and  $z' > L, z'' \leq L$  respectively. Using a suitable finite difference scheme, Equations 30 and 31 along with the above boundary conditions can be written as a set of linear algebraic equations of the form  $A\hat{G} = I$  where  $\hat{G}$  is the correlation function matrix,  $I$  is the unit matrix, and  $A$  is the coefficient matrix. Since matrix  $A$  is a sparse, symmetric, and positive definite matrix it can be inverted efficiently. We used Python's *scipy.sparse.linalg.spsolve* to solve for  $G$ . Furthermore, to calculate the integral in Eq. 32 one can use the Legendre-Gauss quadrature method. As the value of  $\hat{G}$  for one quadrature point will be independent of the other, the integration step can be trivially parallelized. A detailed discussion on efficient ways to invert  $A$  and implement the Legendre-Gauss quadrature method for integration can be found in Z. Xu and A.C. Maggs[5].

- 
- [1] R. R. Netz and H. Orland, [Eur. Phys. J. E](#) **11**, 301 (2003).
  - [2] Z. G. Wang, [Phys. Rev. E](#) **81**, 021501 (2010).
  - [3] N. R. Agrawal and R. Wang, [J. Chem. Theory Comput.](#) **18**, 6271 (2022).
  - [4] N. R. Agrawal and R. Wang, [Phys. Rev. Lett.](#) **129**, 228001 (2022).
  - [5] Z. Xu and A. C. Maggs, [J. Comput. Phys.](#) **275**, 310 (2014).
